# Supplementary material for: pH modulates friction memory effects in protein folding
Source: arXiv:2401.12027 ancillary file (2024-01-22)
Supplement: Supplementary file 1 [file SI.pdf]

# pH modulates memory effects in protein folding - Supplementary Materials

Benjamin A. Dalton and Roland R. Netz
*Freie Universität Berlin, Fachbereich Physik, 14195 Berlin, Germany*

**CONTENTS**

1. Simulation details, analysis, and table of parameters 2

2. Fraction of native contacts reaction coordinate 3

3. Distributions of barrier crossing times 5

4. Memory kernel fitting 7

5. Asymptotic cross-over formula and the Grote-Hynes theory 8

References 10

## 1. SIMULATION DETAILS, ANALYSIS, AND TABLE OF PARAMETERS

The all-atom trajectories for the neutral pH system studied in the main manuscript were previously published by Lindorff-Larsen et al. [1]. The trajectories for the low pH system were previously published by Chung and Piana-Agostinetti et al. [2]. In the latter, all aspartate and glutamate residues are simulated in their protonated states. All simulations were performed using the CHARMM22* force field [3] with a 2 fs time step and the data was stored at 0.2 ns intervals, which is the time resolution for the data analysed in the present manuscript. The influence of the low time resolution of the data was discussed previously [4, 5]. From the all-atom simulation data, we project all trajectories onto the fraction of native contacts reaction coordinate (discussed in Section 2). The non-Markovian memory kernels, and hence the friction, are extracted using methods that are described in detail in Dalton et al. [4]. In Table S1, we present the relevant parameters and time scales extracted from the simulation trajectories. The various definitions of folding times are described below in Section 3. The Markovian predictions ($\tau_{\rm Mar}^{\rm u\to b}$ and $\tau_{\rm Mar}^{\rm u\to f}$) are determined using Eq. 2 in the main manuscript.

TABLE S1. Table of parameters and time scales extracted from simulation trajectories. A distinction is made between transitions between the unfolded state and the top of the free energy barrier ($Q_{\rm u} \to Q_{\rm b}$), and transitions from the unfolded state to the folded state ($Q_{\rm u} \to Q_{\rm f}$). Error estimates for the residency times are for standard errors (see Section 3)

| | low pH | neutral pH | description |
|---|---|---|---|
| $U_0$ [$k_BT$] | 2.6 | 1.7 | folding barrier height |
| $L_{\rm u}^{\rm u\to b}$ | 0.22 | 0.15 | reaction coordinate distance ($Q_{\rm u} \to Q_{\rm b}$) |
| $\gamma$ [$10^{12}$ unm$^2$ns$^{-1}$] | 0.1 | 2.2 | total friction |
| $\tau_{\rm D}$ [$\mu$s] | 1.5 | 16.2 | diffusion time scale ($\tau_{\rm D} = \gamma(Q_{\rm b} - Q_{\rm u})^2/k_{\rm B}T$) |
| $\tau_{\rm mem}$ [$\mu$s] | 0.069 | 3.3 | first-moment memory time |
| $\tau_{\rm Res}^{\rm u\to b}$ [$\mu$s] | 5.5 ± 0.7 | 5.8 ± 0.9 | unfolded state residency times ($Q_{\rm u} \to Q_{\rm b}$) |
| $\tau_{\rm Res}^{\rm u\to f}$ [$\mu$s] | 10.4 ± 2.3 | 24.8 ± 9.9 | unfolded state residency times ($Q_{\rm u} \to Q_{\rm f}$) |
| $N_{\rm Res}^{\rm u\to b}$ | 47 | 52 | number of unfolded state residencies ($Q_{\rm u} \to Q_{\rm b}$) |
| $N_{\rm Res}^{\rm u\to f}$ | 24 | 12 | number of unfolded state residencies ($Q_{\rm u} \to Q_{\rm f}$) |
| $\tau_{\rm MFP}^{\rm u\to b}$ [$\mu$s] | 5.2 | 6.3 | mean first-passage time ($Q_{\rm u} \to Q_{\rm b}$, $\tau_{\rm MFP}^{\rm MD}$ in manuscript) |
| $\tau_{\rm MFP}^{\rm u\to f}$ [$\mu$s] | 11.4 | 32.9 | mean first-passage time ($Q_{\rm u} \to Q_{\rm f}$) |
| $\tau_{\rm Mar}^{\rm u\to b}$ [$\mu$s] | 5.1 | 37.4 | Markovian prediction ($Q_{\rm u} \to Q_{\rm b}$, $\tau_{\rm MFP}^{\rm Mar}$ in manuscript) |
| $\tau_{\rm Mar}^{\rm u\to f}$ [$\mu$s] | 7.0 | 59.5 | Markovian prediction ($Q_{\rm u} \to Q_{\rm f}$) |

## 2. FRACTION OF NATIVE CONTACTS REACTION COORDINATE

**The fraction of native contacts:** For each protein, we project the back-bone $C_\alpha$ atomic positions from the all-atom trajectories onto the fraction of native contacts reaction coordinate $Q$, evaluated with a soft cut-off potential [6]. The evaluation of $Q(t)$ requires a reference state, which we take to be the native state for each trajectory. To evaluate the native state, we select from amongst the member states of the trajectories. The approach is similar to that used by Lindorff-Larsen *et. al.* [1] and Best *et. al.* [6], which follows from [7]. We sample a subset of evenly spaced states from the full trajectory. For each pair of states, we calculate the corresponding root-mean-squared deviation (RMSD) between the two states. If the RMSD between two states is less than 0.2 nm, then we place the pair into a list. We assign the state that has the most listed pairs satisfying the RMSD condition as the native state for a given protein. We select a single native state from amongst the two trajectory segments for each protein system, which we then use for all segments. In the native state, we define all $C_\alpha$ pairs that are separated by at least 5 residues in the primary sequence and which are separated by less than 0.9 nm in Cartesian distance, as the native contacts. Each protein will have $N_{\mathrm{nc}}$ native contacts. $\mathbf{s}^0_{ij}$ are the separation vectors for all native contact pairs in the native state, which have magnitudes $s^0_{ij} = \sqrt{\mathbf{s}^0_{ij} \cdot \mathbf{s}^0_{ij}}$. $\mathbf{s}_{ij}(t)$ are the separation vectors for all native contact pairs at each time, with magnitudes $s_{ij}(t) = \sqrt{\mathbf{s}_{ij}(t) \cdot \mathbf{s}_{ij}(t)}$. This gives the fraction of the native contacts that are deemed to be in contact at time t as

$$Q(t) = \frac{1}{N_{\mathrm{nc}}} \sum_{i<j} \frac{1}{1 + \mathrm{e}^{\beta(s_{ij}(t) - \gamma s^0_{ij})}}, \tag{S1}$$

where the summation indices $i$ and $j$ are only for native contact pairs. Here, we set the parameters such that $\beta = 30$ nm$^{-1}$ and $\gamma = 1.6$.

In Figs. S1A and B, we show the full $Q(t)$ trajectories for $\alpha$3D under both pH conditions. The probability densities, accumulated by compiling both trajectory segments for a given system, are given in Figs. S1C. In the main manuscript, we discuss the quality of $Q$ as a reaction coordinate, evaluated by the Bayesian formula for the transition-path probability [8]:

$$P(TP|Q) = \frac{P(Q|TP)P(TP)}{P(Q)}. \tag{S2}$$

Fig. S1D, we show $P(Q|TP)$, which is extracted from simulation. In Fig. S1E, we show the resulting $P(TP|Q)$. In the main manuscript, we show Figs. S1E with a shifted and rescaled $Q$-axis, such that we can compare $P(TP|Q)$ between the two systems.

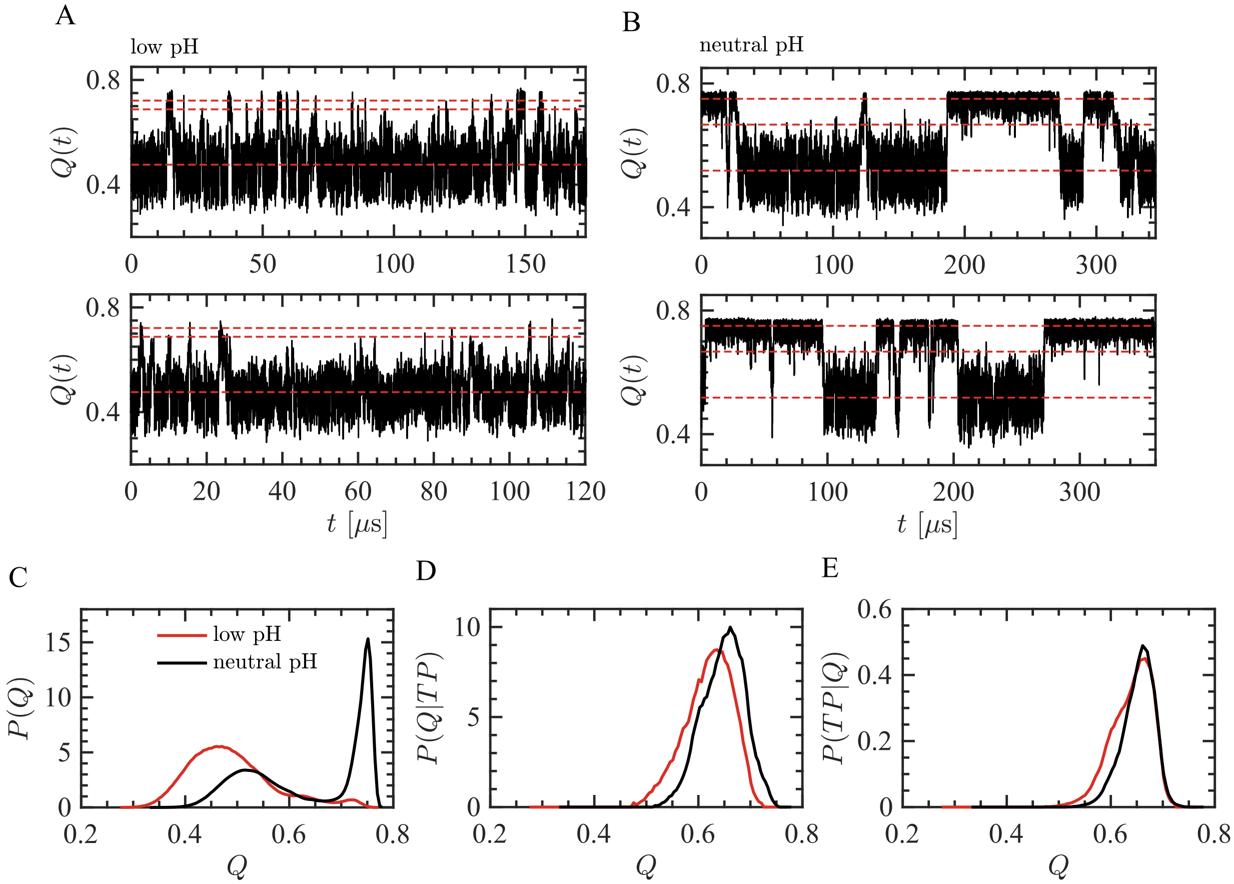


FIG. S1. Additional material for the fraction of native contacts reaction coordinate for the $\alpha$3D protein under low-pH and neutral-pH conditions. A) Two full independent trajectories for $\alpha$3D under the low-pH condition. Total simulation time is 295 $\mu$s [2]. B) Two full independent trajectories for $\alpha$3D under the neutral-pH condition. Total simulation time is 707 $\mu$s [1, 2]. C) Total probability density for $Q$ ($P(Q)$) under both conditions. D) The probability of being at position $Q$ given that the protein is on a transition path $P(Q|TP)$. E) The Bayesian criteria for the conditional probability to be on a transition path, given that the reaction coordinate is at $Q$. This criterium is calculated using the Bayesian formula (Eq. S2). C, D, and E are evaluated by compiling the two trajectories in A and B for each condition.

## 3. DISTRIBUTIONS OF BARRIER CROSSING TIMES

In this section, we describe the various definitions of folding times and present the folding time distributions for each definition. In Fig. S2, we provide a schematic for the various definitions. A common method to evaluate a folding time is to evaluate the mean residency time, i.e. the average time spent in the unfolded state, beginning when the system first enters into the unfolded state ($Q_\mathrm{u}$) and ending when it first reaches the folded state ($Q_\mathrm{f}$). An individual residency time is indicated by the $Q_\mathrm{u} \to Q_\mathrm{f}$ residency transition in Fig. S2. A residency time can be also defined for transitions from the unfolded state to the barrier top (indicated by the $Q_\mathrm{u} \to Q_\mathrm{b}$ residency). Likewise, we can calculate the sequence of first-passage times from both $Q_\mathrm{u} \to Q_\mathrm{f}$, and $Q_\mathrm{u} \to Q_\mathrm{b}$.

In Fig. S3, we show the non-normalized distributions for all folding times for $\alpha$3D. The mean values are given in Table S1 and the standard deviations $\sigma$ are presented within each figure panel. Despite the long simulation trajectories, residency times for $Q_\mathrm{u} \to Q_\mathrm{f}$ are not particularly well sampled and incur large errors due to small sample numbers (Table S1). The errors are significantly reduced for $Q_\mathrm{u} \to Q_\mathrm{b}$ residency times. This is a consequence of barrier recrossing effects, which occur because the $Q$ reaction coordinate exhibits strong non-Markovianity. A sequence of first-passage times is strongly correlated. Therefore, the estimation of errors for mean first-passage times are far less straightforward. We see, however, that standard deviations for both residency times and first-passage times are in good agreement.

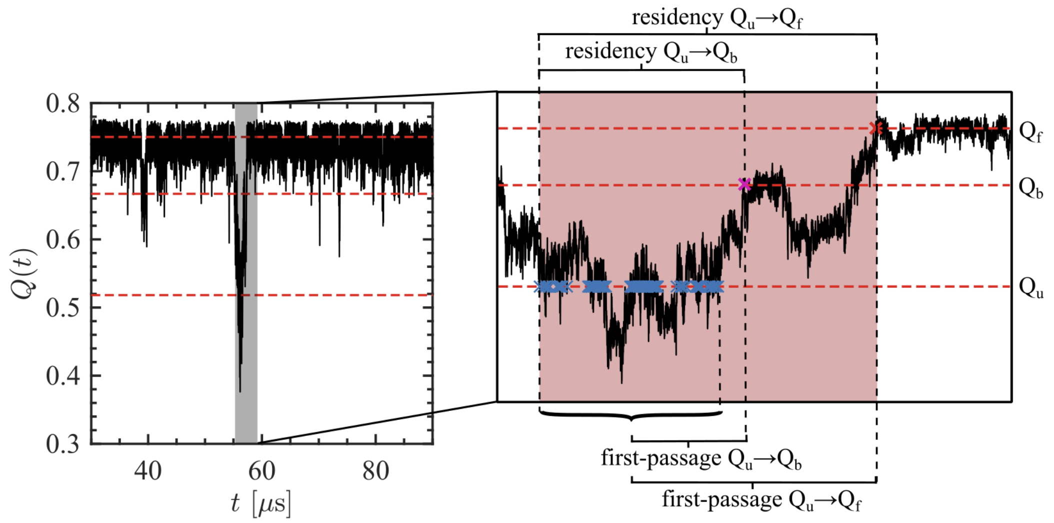


FIG. S2. Schematic showing the various definitions of folding times. The red box shows an example of a residency time, which is the time between a new arrival in the unfolded state $Q_\mathrm{u}$ and the subsequent arrival in the folded state $Q_\mathrm{f}$. The blue crosses show a sequence of crossings of the unfolded state minimum. The first-passage times to the barrier top are the time between each blue cross and the magenta cross at $Q_\mathrm{b}$. The first-passage times to the folded state are the time between each blue cross and the red cross at $Q_\mathrm{f}$.

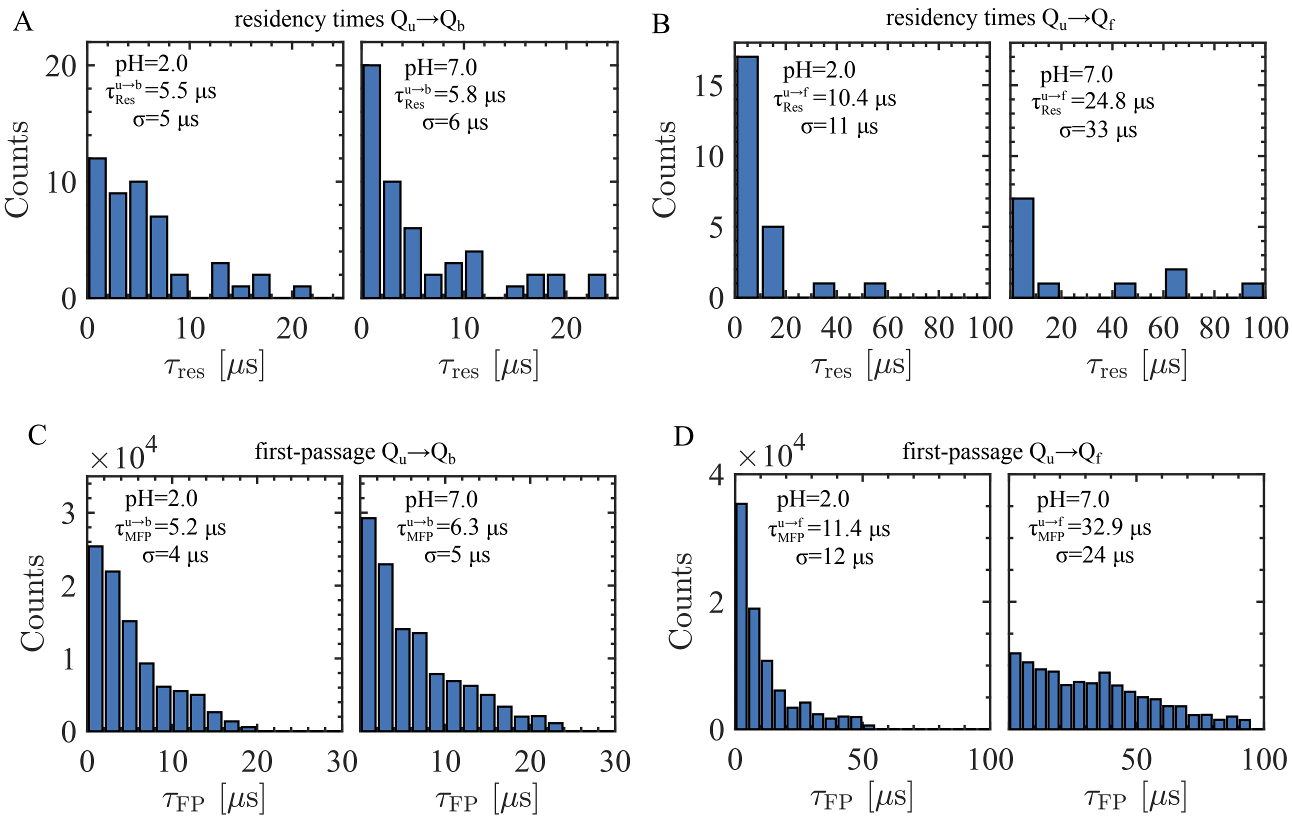


$\tau_{\mathrm{Res}}^{\mathrm{u}\to\mathrm{b}}$=4 μs $\quad$ $\tau_{\mathrm{MFP}}^{\mathrm{u}\to\mathrm{b}}$=4 μs

$\tau_{\mathrm{Res}}^{\mathrm{u}\to\mathrm{f}}$=4 μs $\quad$ $\tau_{\mathrm{MFP}}^{\mathrm{u}\to\mathrm{f}}$=4 μs

FIG. S3. Distributions, means, and standard deviations for various definitions of folding times. See Fig. S2 for a description of each folding time definition. A) and B) show histograms of unfolded-state residency times, defined for both $Q_{\mathrm{u}} \to Q_{\mathrm{b}}$ and $Q_{\mathrm{u}} \to Q_{\mathrm{f}}$. The total number of events is given in Table S1, as are the mean values and the standard errors. C) first-passage time histograms for transitions from the unfolded state to the barrier top ($Q_{\mathrm{u}} \to Q_{\mathrm{b}}$). D) The first-passage time distributions for the unfolded state to the folded state ($Q_{\mathrm{u}} \to Q_{\mathrm{f}}$). Mean first-passage times are given in Table S1. Mean values for C) are the $\tau_{\mathrm{MFP}}^{\mathrm{MD}}$ values that appear in the main manuscript.

## 4. MEMORY KERNEL FITTING

TABLE S2. Table of fitting parameters for $\alpha$3D memory kernels. Fit expressions are given by $\Gamma(t) = \sum_{n=1}^{4} \gamma_n \mathrm{e}^{-t/\tau_n}/\tau_n$. Memory times $\tau_n$ are given in units of [$1\times10^3$ ns] and pre-factors $\gamma_n$ are in units of [$1\times10^{11}$unm$^2$ns$^{-1}$]. Total friction is given by $\gamma = \sum_{n=1}^{4} \gamma_n$ and the mean memory time $\tau_{\mathrm{mem}}$ is the first moment of the memory kernel $\tau_{\mathrm{mem}} = \int_0^\infty t\Gamma(t)dt / \int_0^\infty \Gamma(t)dt$.

| | $\gamma_1$ | $\tau_1$ | $\gamma_2$ | $\tau_2$ | $\gamma_3$ | $\tau_3$ | $\gamma_4$ | $\tau_4$ | $\gamma$ | $\tau_{\mathrm{mem}}$ |
|---|---|---|---|---|---|---|---|---|---|---|
| pH = 2.0 | 0.49 | 0.12 | 0.34 | $3.0\times10^{-2}$ | 0.11 | $3.5\times10^{-3}$ | 0.04 | $6.0\times10^{-4}$ | 0.98 | 0.067 |
| pH = 7.0 | 19.4 | 3.9 | 2.44 | $6.3\times10^{-2}$ | 0.55 | $6.6\times10^{-3}$ | 0.17 | $8.0\times10^{-4}$ | 22.6 | 3.4 |

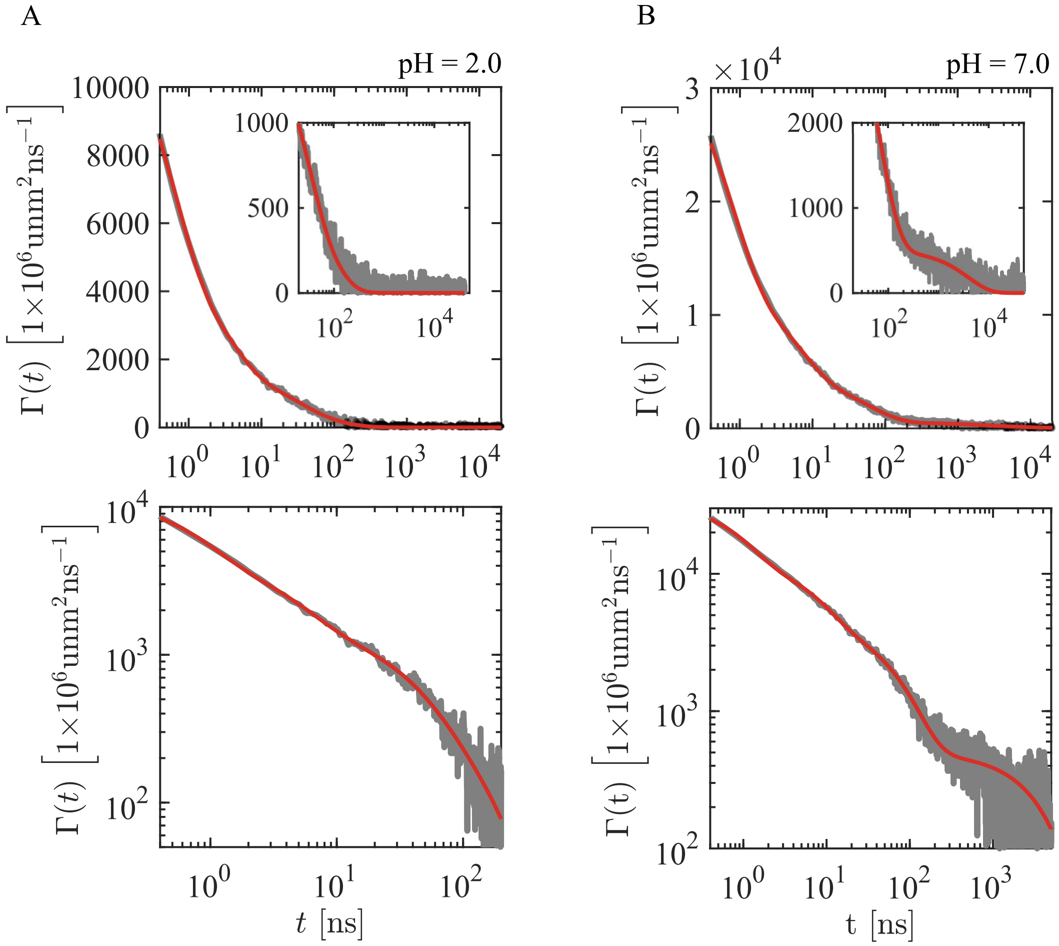


FIG. S4. Memory kernels extracted for the $Q$ reaction coordinate for $\alpha$3D under low pH condition (A) and neutral pH condition (B) with fitting results. Memory kernels are fit with a 4-component exponential series $\Gamma(t) = \sum_{n=1}^{4} \gamma_n \mathrm{e}^{-t/\tau_n}/\tau_n$, shown in red. Insets in the top panels show magnifications of the long-time-tail behaviour for each memory kernel and for the fitting. The bottom panels show the same data on a log-log scale.

## 5. ASYMPTOTIC CROSS-OVER FORMULA AND THE GROTE-HYNES THEORY

**Asymptotic cross-over formula:** For a non-Markovian system in 1D with a multi-exponential memory kernel given by $\Gamma(t) = \sum_{i=1}^{N} \gamma_i e^{-t/\tau_i}/\tau_i$ we can use a previously published asymptotic cross-over formula [9–11] to predict the barrier crossing time $\tau^{\mathrm{asy}} = \tau^{\mathrm{asy}}(\tau_{\mathrm{D}}, U_0, \{\gamma_i\}, \{\tau_i\}, \tau_{\mathrm{m}})$, where $\tau_{\mathrm{m}} = m/\gamma$, $\tau_{\mathrm{D}} = \gamma(Q_{\mathrm{b}} - Q_{\mathrm{u}})^2/k_{\mathrm{B}}T$, $\{\gamma_i\}$ and $\{\tau_i\}$ are the set of $N$ friction pre-factors and times scales, such that $\gamma = \sum_{i=1}^{N} \gamma_i$, and $U_0$ is the barrier height. There are $N$ overdamped contributions ($\tau^i_{\mathrm{OD}}$) and $N$ energy-diffusion contributions ($\tau^i_{\mathrm{ED}}$). The overdamped contributions are given by

$$\tau^i_{\mathrm{OD}} = \tau_{\mathrm{D}} \frac{\gamma_i}{\gamma} \frac{e^{\beta U_0}}{\beta U_0} \left[ \frac{\pi}{4\sqrt{2}} \frac{1}{1 + 10\beta U_0 \tau_i/\tau_{\mathrm{D}}} + \sqrt{\beta U_0 \frac{\tau_{\mathrm{m}}}{\tau_{\mathrm{D}}}} \right], \tag{S3}$$

where an additional factor of 1/2 has been included in the first term to account for transitions that only pass from a state minimum to the barrier top. The energy diffusion contributions are given by

$$\tau^i_{\mathrm{ED}} = \tau_{\mathrm{D}} \frac{\gamma}{\gamma_i} \frac{e^{\beta U_0}}{\beta U_0} \left[ \frac{\tau_{\mathrm{m}}}{\tau_{\mathrm{D}}} + 4\beta U_0 \left( \frac{\tau_i}{\tau_{\mathrm{D}}} \right)^2 + \sqrt{\beta U_0 \frac{\tau_{\mathrm{m}}}{\tau_{\mathrm{D}}}} \right]. \tag{S4}$$

The predicted barrier crossing time is then given by

$$\tau^{\mathrm{asy}}(\tau_{\mathrm{D}}, U_0, \{\gamma_i\}, \{\tau_i\}, \tau_{\mathrm{m}}) = \sum_{i=1}^{4} \tau^i_{\mathrm{OD}} + \left[ \sum_{i=1}^{4} \frac{1}{\tau^i_{\mathrm{ED}}} \right]^{-1}. \tag{S5}$$

In the Markovian limit, i.e. $\tau_i \to 0$ for all memory time scales, Eq. S5 reduces to

$$\tau^{\mathrm{asy}}_{\mathrm{Mar}}(\tau_{\mathrm{D}}, U_0, \{\gamma_i\}, 0, \tau_{\mathrm{m}}) = \tau_{\mathrm{D}} \frac{e^{\beta U_0}}{\beta U_0} \left[ \frac{\pi}{2\sqrt{2}} + 2\sqrt{\beta U_0 \frac{\tau_{\mathrm{m}}}{\tau_{\mathrm{D}}}} + \frac{\tau_{\mathrm{m}}}{\tau_{\mathrm{D}}} \right]. \tag{S6}$$

Furthermore, we see that in the high-friction, Markovian (HF) limit, i.e. when additionally $\tau_{\mathrm{m}} \to 0$, we obtain from Eq. S6

$$\tau^{\mathrm{asy}}_{\mathrm{HF}} = \tau^{\mathrm{asy}}_{\mathrm{Mar}}(\tau_{\mathrm{D}}, U_0, \{\gamma_i\}, 0, 0) = \tau_{\mathrm{D}} \pi e^{\beta U_0}/4\beta U_0 \sqrt{2}. \tag{S7}$$

We can multiple all memory time scales that enter into Eq. S5 by a common factor $\alpha$. This results in an effective $\alpha$-dependent memory kernel $\Gamma^{\alpha}(t)$, and corresponding first-moment memory time $\alpha\tau_{\mathrm{mem}}$:

$$\Gamma_{\alpha}(t) = \sum_{i=1}^{N} \frac{\gamma_i}{\alpha\tau_i} \exp\left(t/\alpha\tau_i\right), \quad \alpha\tau_{\mathrm{mem}} = \int_0^{\infty} t\Gamma_{\alpha}(t)dt \Big/ \int_0^{\infty} \Gamma_{\alpha}(t)dt, \tag{S8}$$

Likewise, this results in $\alpha$-dependent overdamped and energy-diffusion components, which are given by

$$\begin{aligned} \tau^i_{\alpha,\mathrm{OD}} &= \tau_{\mathrm{D}} \frac{\gamma_i}{\gamma} \frac{e^{\beta U_0}}{\beta U_0} \left[ \frac{\pi}{2\sqrt{2}} \frac{1}{1 + 10\beta U_0 \alpha\tau_i/\tau_{\mathrm{D}}} + \sqrt{\beta U_0 \frac{\tau_{\mathrm{m}}}{\tau_{\mathrm{D}}}} \right] \\ \tau^i_{\alpha,\mathrm{ED}} &= \tau_{\mathrm{D}} \frac{\gamma}{\gamma_i} \frac{e^{\beta U_0}}{\beta U_0} \left[ \frac{\tau_{\mathrm{m}}}{\tau_{\mathrm{D}}} + 4\beta U_0 \left( \alpha\frac{\tau_i}{\tau_{\mathrm{D}}} \right)^2 + \sqrt{\beta U_0 \frac{\tau_{\mathrm{m}}}{\tau_{\mathrm{D}}}} \right]. \end{aligned} \tag{S9}$$

The $\alpha$-dependent asymptotic cross-over formula is $\tau^{\mathrm{asy}}_{\alpha} = \tau^{\mathrm{asy}}(\tau_{\mathrm{D}}, U_0, \{\gamma_i\}, \{\alpha\tau_i\}, \tau_{\mathrm{m}})$. Since Eq. S7 does not depend on $\alpha$, $\tau^{\mathrm{asy}}_{\alpha}/\tau^{\mathrm{asy}}_{\mathrm{HF}}$ is given by

$$\frac{\tau^{\mathrm{asy}}_{\alpha}}{\tau^{\mathrm{asy}}_{\mathrm{HF}}} = \frac{2\beta U_0\sqrt{2}}{\tau_{\mathrm{D}} \pi e^{\beta U_0}} \tau^{\mathrm{asy}}(\tau_{\mathrm{D}}, U_0, \{\gamma_i\}, \{\alpha\tau_i\}, \tau_{\mathrm{m}}), \tag{S10}$$

which appears in the main manuscript.

**Grote-Hynes theory:** The transition state theory (TST) barrier-crossing time is given by

$$\tau^{\rm TST} = \frac{2\pi}{\omega_{\rm min}} e^{\beta U_0} \tag{S11}$$

where $\omega_{\rm min} = \sqrt{U''_{\rm min}/m}$ is the frequency at the free-energy minimum. The Grote-Hynes (GH) prediction for the barrier-crossing time is given by

$$\tau^{\rm GH} = \frac{\omega_{\rm max}}{\lambda} \tau^{\rm TST} = \frac{2\pi\omega_{\rm max}}{\lambda\omega_{\rm min}} e^{\beta U_0}, \tag{S12}$$

where $\omega_{\rm max} = \sqrt{|U''_{\rm max}|/m}$ is the frequency at the free-energy barrier top. $U''_{\rm min}$ and $U''_{\rm max}$ are the free energy curvatures at the minimum and maximum and $m$ is the mass of the particle. $\lambda$ is the barrier reactive frequency, which is determined by solving the Grote-Hynes equation

$$\lambda^2 + \lambda \frac{\tilde{\Gamma}(\lambda)}{m} = \omega_{\rm max}^2. \tag{S13}$$

$\tilde{\Gamma}(\lambda)$ is the Laplace transform of the friction memory kernel, given by

$$\tilde{\Gamma}(\lambda) = \int_0^\infty \Gamma(t') e^{-\lambda t'} dt'. \tag{S14}$$

Having obtained $\tilde{\Gamma}(\lambda)$, one then solves Eq. S13, which will have one real and positive root. This root is assigned as the reactive frequency $\lambda$, which enters into Eq. S12. In the Markovian limit, $\Gamma(t) = \gamma\delta(t)$ and hence $\tilde{\Gamma}(\lambda) = \gamma$, $\tau^{\rm GH}$ reduces to the Kramers barrier crossing time $\tau^{\rm GH}_{\rm Kr}$ for medium-to-high friction, which is given by

$$\tau^{\rm GH}_{\rm Kr} = \left[ \sqrt{\frac{\gamma^2}{4m^2} + \omega_{\rm max}^2} - \frac{\gamma}{2m} \right]^{-1} \omega_{\rm max} \tau^{\rm TST}. \tag{S15}$$

In the high-friction (HF) limit, we can further reduce the prediction Eq. S15 to

$$\tau^{\rm GH}_{\rm HF} = \frac{\gamma}{m\omega_{\rm max}} \tau_{\rm TST}. \tag{S16}$$

Similar to Eq. S8, we introduce the uniform $\alpha$ rescaling by replacing the Laplace transform in Eq. S14 with a Laplace transform of the rescaled memory kernel (Eq. S8)

$$\tilde{\Gamma}^\alpha(\lambda) = \int_0^\infty \Gamma^\alpha(t') e^{-\lambda t'} dt', \tag{S17}$$

and hence evaluate $\lambda^2 + \lambda\tilde{\Gamma}^\alpha(\lambda)/m = \omega_{\rm max}^2$ over the range of $\alpha$, leading to $\tau_\alpha^{\rm GH}$. Combining with Eq. S16 gives $\tau_\alpha^{\rm GH}/\tau_{\rm HF}^{\rm GH}$, which appears in the main manuscript.

[1] K. Lindorff-Larsen, S. Piana, R. O. Dror, and D. E. Shaw, Science **334**, 517 LP (2011).
[2] H. S. Chung, S. Piana-Agostinetti, D. E. Shaw, and W. A. Eaton, Science (New York, N.Y.) **349**, 1504 (2015).
[3] S. Piana, K. Lindorff-Larsen, and D. E. Shaw, Biophysical journal **100**, L47 (2011).
[4] B. A. Dalton, C. Ayaz, H. Kiefer, A. Klimek, L. Tepper, and R. R. Netz, Proceedings of the National Academy of Sciences **120**, e2220068120 (2023).
[5] L. Tepper, B. A. Dalton, and R. R. Netz, arXiv (2024), arXiv.2401.09249.
[6] R. B. Best, G. Hummer, and W. A. Eaton, Proceedings of the National Academy of Sciences **110**, 17874 LP (2013).
[7] X. Daura, K. Gademann, B. Jaun, D. Seebach, W. F. van Gunsteren, and A. E. Mark, Angewandte Chemie International Edition **38**, 236 (1999).
[8] G. Hummer, New Journal of Physics **7**, 34 (2005).
[9] J. Kappler, J. O. Daldrop, F. N. Brünig, M. D. Boehle, and R. R. Netz, The Journal of Chemical Physics **148**, 14903 (2018).
[10] J. Kappler, V. B. Hinrichsen, and R. R. Netz, The European Physical Journal E **42**, 119 (2019).
[11] L. Lavacchi, J. Kappler, and R. R. Netz, EPL **131** (2020).
